# Supplementary material for: Closing the Gap: Achieving Global Convergence (Last Iterate) of Actor-Critic under Markovian Sampling with Neural Network Parametrization
Source: arXiv:2405.01843 source file (2024-12-09)
Supplement: Supplementary file 1 [file problem_setup_supplement.tex]

\section{Problem Setup Continued}\label{setup_supp}

We define the Bellman operator for a policy $\pi$ as follows
\begin{equation}
(T^{\pi}Q)(s,a) =  r(s,a) + \gamma \int Q^{\pi}(s',\pi(s'))P(ds'|s,a), \label{ps_3}
\end{equation}
where $r(s,a) = \mathbb{E}(r'(s,a)|(s,a))$ Similarly we define the Bellman Optimality Operator as 

Similarly we define the Bellman Optimality Operator as  
\begin{equation}
(TQ)(s,a) = \left(r(s,a) +\max_{a' \in \mathcal{A}}\gamma\int Q(s',a')P(ds'|s,a)\right),\label{ps_4}
\end{equation}

Further, operator $P^{\pi}$ is  defined as
\begin{equation}
P^{\pi}Q(s,a)=\mathbb{E}[Q(s',a')|s' \sim P(\cdot|s,a), a' \sim \pi(\cdot|s') ]\label{ps_7} ,    
\end{equation}
which is the one step Markov transition operator for policy $\pi$ for the Markov chain defined on $\mathcal{S}\times\mathcal{A}$ with the transition dynamics given by $S_{t+1} \sim P(\cdot|S_{t},A_{t})$ and $A_{t+1} \sim \pi(\cdot|S_{t+1})$. It defines a distribution on the state action space after one transition from the initial state. Similarly, $P^{\pi_{1}}P^{\pi_{2}}\cdots{P}^{\pi_{m}}$ is the $m$-step Markov transition operator following policy $\pi_t$ at steps $1\le t\le m$. It defines a distribution on the state action space after $m$ transitions from the initial state. We have the relation 
\begin{eqnarray}
(T^{\pi}Q)(s,a) &=&  r(s,a) + \gamma \int Q^{\pi}(s',\pi(s'))P(ds'|s,a) \nonumber\\
           &&     \label{ps_7_2}\\
         &=&  r(s,a) + {\gamma}(P^{\pi}Q)(s,a)
\end{eqnarray}

We thus defines $P^{*}$ as 
\begin{equation}
P^{*}Q(s,a)=\max_{a^{'} \in \mathcal{A}}\mathbb{E}[Q(s',a')|s' \sim P(\cdot|s,a)]\label{ps_7_3} ,
\end{equation}
in other words, $P^{*}$ is the one step Markov transition operator with respect to the greedy policy of the function on which it is acting.

For any measurable function $f:\mathcal{S}\times\mathcal{A}:\rightarrow\mathbb{R}$, we also define 
\begin{equation}
\mathbb{E}(f)_{\nu}=\int_{\mathcal{S}\times\mathcal{A}}fd\nu,  
\end{equation}
for any distribution $\nu\in\mathcal{P}(\mathcal{S}\times\mathcal{A})$.

%\subsection{ Deep Network Parameter Estimation for 2-layer NN with ReLU activation } \label{ Deep Network Parameter Estimation for 2-layer NN with ReLU activation }
